# Supplementary material for: Game Semantics: Easy as Pi
Source: arXiv:2011.05248 source file (2020-11-10)
Supplement: Supplementary file 1 [file appendix-det.tex]

%! TEX root = main.tex

\section{Proofs of \S~\ref{sec:det}}

\subsection{Proofs of \S~\ref{sec:detstrat}}
\adjunt*
\begin{proof}
  The adjunction is fairly simple to describe:
  \begin{itemize}
  \item From $ \sigma : \LiftPlus A \profto B$ in $\DetStrat^+$, by removing
    the initial negative event on $\LiftPlus A$, we get a strategy
    $A \profto B$ in $\DetStrat$ (not necessarily negative).
  \item From $ \sigma : A \profto B$ in $\DetStrat$, we can build a strategy
    $\mathbf{box}^- \cdot  \sigma  : \LiftPlus A \profto B$ which is
    well-defined because $B$ is positive.
  \end{itemize}
  It is clear that these operations are inverse of each other;
  naturality is a simple calculation.
\end{proof}

\subsection{Proofs of correctness of the call-by-name
translation}\label{sec:det-call-by-name-proof}

\subsubsection{Definition of $ \rightarrow _{\PCF}$} First, we define exhaustively $ \rightarrow _{\PCF}$:
\begin{mathpar}
  \infer{( \lambda x.\, M)\, N  \rightarrow_{\PCF}  M \subst x N} {}
  \and
  \infer{\ifte \ttrue M N  \rightarrow_{\PCF}  M} {}
  \and
  \infer{\ifte \ffalse M N  \rightarrow_{\PCF}  N} {}
  \and
  \infer{\texttt{iszero}(0)  \rightarrow_{\PCF}  \ttrue} {}
  \and
  \infer{\texttt{iszero}(n)  \rightarrow_{\PCF}  \ffalse} {n > 0}
  \and
  \infer{\texttt{succ}(n)  \rightarrow_{\PCF}  n+1} {}
  \and
  \infer{Y\, M  \rightarrow_{\PCF}  M\, (Y\, M)} {}
  \and
  \infer{E[M]  \rightarrow_{\PCF}  E[M']} {M  \rightarrow_{\PCF}  M'}
\end{mathpar}
where $E[]$ is an evaluation context, defined by the following grammar:
$$E[] ::= [] \mid E\, N \mid  \lambda x. E \mid \mathtt{iszero}(E) \mid \mathtt{succ}(E) \mid \ifte E M N.$$

First, it is straightforward to extend the substitution lemma in this
setting:

\begin{lemma}[Substitution lemma]\label{lemma:sub_pcf}
  Let $ \Gamma , x:  \sigma   \vdash  M :  \tau $ and $ \Gamma   \vdash  N :  \sigma $. We have
  $$\transl{M\subst x N}^o_i \similarProcesses \shareInteract x y {\transl  \Gamma } {\transl M^o_i} {\Prom y r.\, \transl N^r}.$$
\end{lemma}
\begin{proof}
  By induction on $M$.
\end{proof}
\begin{lemma}[Soundness]\label{lemma:soundnessPCF}
  For $ \Gamma   \vdash  M, N :  \tau $, if $M \rightarrow_{\PCF} N$, then
  $\transl M^o \similarProcesses \transl N^o$.
\end{lemma}
\begin{proof}
  The proof is essentially the same as for the affine case, by simple
  application of the equational rules.

  Let us detail a few rules. First, it is enough to show that
  $\transl M^o_i \similarProcesses \transl N^o_i$ for all
  $i \in \CompType  \tau $.
  \begin{itemize}
  \item $ \beta $-reduction:
    $$
    \begin{aligned}
      \transl {( \lambda x.\, M)\, N}^o_i
      &\similarProcesses
      \shareInteract x y {\transl  \Gamma }
      {\Split o {x, o} {\Naming o {x, o}.\, \transl M^o_i}}
      {\Prom y r.\, \transl N^r} \\
      &\similarProcesses
      \transl {M \subst x N}^o_i
    \end{aligned}$$
    by direct application of Lemma \ref{lemma:sub_pcf}.
  \item if:
    $$
    \begin{aligned}
      \transl {\ifte \ttrue M N}^o_i
      &\similarProcesses
      \shareInteract u v {\transl { \Gamma }}
      {\Output u \ttrue}
      {\InputII v {} {\ttrue: \transl M^o_i; ...}} \\
      &\similarProcesses \transl M^o_i
    \end{aligned}$$
  \item succ:
    $$\transl {\mathtt{succ}(n)}^o_\Start
    \similarProcesses
    \shareInteract x y {}
    {\Output x n}
    {\InputII y {} {\Output o {n+1}}} \similarProcesses \Output o {n+1}$$
  \end{itemize}
\end{proof}

\subsubsection{Finitary PCF and adequacy} Let us define finitary PCF here as the
subset of PCF without fixpoint, with an added term $\bot : A$ denoting
formal divergence. Closed terms of finitary PCF of type $ \mathbb{N} $ converge
either towards a natural number or towards $\bot$ in a finite number
of step. Given a term of PCF $M$, we write its $n$-th approximation
$M_n$ defined as $M$ where $Y$ is substituted by $ \lambda f.\, f^n\, \bot$
where $f^n$ is the $n$-fold iteration of $f$.

\begin{lemma}
  $\transl M^o$ is the limit of the increasing chain $\transl {M_n}^o$.
\end{lemma}
\begin{proof}
  Straightforward since $Y$ is the limit of the $ \lambda f.\, f^n\, \bot$.
\end{proof}

\begin{lemma}
  For $ \vdash  M :  \mathbb{N} $, if $ \llbracket M \rrbracket =  \llbracket n \rrbracket$, then $ \llbracket M_k \rrbracket =  \llbracket n \rrbracket$ for some $k \in  \mathbb{N} $.
\end{lemma}
\begin{proof}
  Trivial, because we know that a positive event labelled $n$ belongs
  to $ \llbracket M \rrbracket$, and since $ \llbracket M \rrbracket$ is the limit of the $ \llbracket M_n \rrbracket$ by the
  previous lemma, and continuity of $ \llbracket \cdot \rrbracket$, the result follows.
\end{proof}
\begin{lemma}\label{lemma:pcf_div_empty}
  If $M$ diverges for $ \rightarrow _{\PCF}$, then
  $\transl M^o \similarProcesses \EmptyProcess$.
\end{lemma}
\begin{proof}
  Since $M$ diverge, we have $M_n  \rightarrow ^*_{\PCF} \bot$ for all $n  \in 
   \mathbb{N} $. Since $\transl {M_n}^o \similarProcesses
  \EmptyProcess$, we can conclude.
\end{proof}
\PCFad*
\begin{proof}
  We already have proved soundness. For adequacy, it is a consequence
  of the previous lemma:
  $M$ cannot diverge, so it must converge to a natural number, and
  clearly the model is injective on natural numbers: $\transl n =
  \transl m$ implies that $n = m$.
\end{proof}

\subsection{Proof of correctness of the call-by-value translation}
First, let us define the relation $ \rightarrow _v$ as the subset of $ \rightarrow _{\PCF}$
which contains only the instances of the $ \beta $-reduction
$( \lambda x.\, M)  \rightarrow  M \subst x N$ when $N$ is a value, ie. a $ \lambda $-abstraction,
a natural number or a boolean.

\valueChar*
\begin{proof}
  Easy case distinction on $N$.
\end{proof}

\subCbv*
\begin{proof}
  By induction on $M$.
\end{proof}

\cbvSound*
\begin{proof}
  Soundness is an easy verification, using Lemma \ref{lemma:subCbv}.

  For adequacy, assume that $ \llbracket M \rrbracket \similarProcesses  \llbracket n \rrbracket$. Because there
  is no recursion, we can normalise $M$ to a term containg
  $\bot$. Actually, it is easy to see that a normal form of type $ \mathbb{N} $
  is either a natural number, or a term of the form $E[\bot]$. Now, by
  induction, we can derive that
  $\transl {E[\bot]}^o_{\vec k} \similarProcesses \EmptyProcess$,
  which is a contradiction since $ \llbracket E[\bot] \rrbracket =  \llbracket M \rrbracket$ must not be empty.
\end{proof}

%%% Local Variables:
%%% mode: latex
%%% TeX-master: "main"
%%% End:
