# Supplementary material for: Game Semantics: Easy as Pi
Source: arXiv:2011.05248 source file (2020-11-10)
Supplement: Supplementary file 2 [file appendix-lindet.tex]

%! TEX root = main.tex
\section{Proofs of \S~\ref{sec:lindetgames}}
In this section, we provide more details proofs of the results
presented in \S~\ref{sec:lindetgames}.

\subsection{Categorical Structure}

\subsubsection{Lifting of Maps to Strategies}
First, let us show some properties of the lifting of maps defined in
\S~\ref{sec:lindet cat}.

Given a "strategy" $ \sigma  : S  \rightarrow  A^\perp  \parallel  B$ and a "map of games"
$f: B  \rightarrow  C$, we form the strategy
$ \sigma _f : S  \downarrow  V  \rightarrow  A^\perp  \parallel  \dom f \xrightarrow{A^\perp  \parallel  f} A^\perp  \parallel  C$
where $V$ contains the set of $s  \in  S$ such that $ \sigma \, s  \in  A  \parallel  \dom f$.

\begin{lemma}
  $ \sigma _f$ is a "strategy" $A \profto C$.
\end{lemma}
\begin{proof}
  Courtesy and determinism follow from $f$ preserving the causal order and
  receptivity from $f$ being bijective on its domain. 
\end{proof}
It is easy to see that $\Lift f$ is equal to $(\cc_A)_f$. We have the following result:

\begin{lemma}\cite{cg1}
  Given $ \sigma  : A \profto B$ and $f : B  \rightarrow  C$ a "map of games", we have:
  $$ \sigma _f  \cong  \Lift f  \odot   \sigma .$$
\end{lemma}

This result implise the functoriality of $\Lift {-}$:
$\Lift {g \circ f} = \Lift g  \odot  \Lift f$.

\subsubsection{Weak products} We now show that $\LinDet$ has weak
products.

\productLinDet*
\begin{proof}
  Consider $ \sigma  : S  \rightarrow  A^\perp  \parallel  B$ and $ \tau  : T  \rightarrow  A^\perp  \parallel  C$. By prefixing, we obtain maps of event structures (but not strategies):
  $$\Left^- \cdot  \sigma  : \Right^- \cdot  \sigma   \rightarrow  A^\perp  \parallel  B \with C \qquad
  \Right^- \cdot  \tau  : \Left^- \cdot  \tau   \rightarrow  A^\perp  \parallel  B \with C$$ Then, it
  is easy to see that their sum forms a map of event structure
  $ \sigma  \sqcup  \tau  : (\Left^- \cdot  \sigma ) + (\Right^- \cdot  \sigma )  \rightarrow  A^\perp  \parallel  (B
  \with C)$.

  An easy verification shows that
  $ \pi _1 \circ ( \sigma \sqcup \tau ) = \sigma $ and similarly for
  $ \pi _2$. To get $\Pairing { \sigma , \tau }$, we precompose with
  copycat to get a strategy, and this operation preserves the
  equations with the projections.
\end{proof}
\subsection{Reasoning on the equational theory}
\label{app:lindetprocess}
In this section, we provide proofs of properties on the equational theory.
%\soundness*
\begin{proof}
  Rules in the compact-close fragment of the theory follow from the
  compact-closed structure of $\LinDet$, in particular bifunctoriality
  of $\parallel$.

  Rules for permutations follow from bifunctoriality of $\parallel$
  and the fact that nested pairing commute (by receptivity).

  In communication, the rules follow from the weak coproduct
  structure. In cut elimination, from an easy investigation on the
  composition.
\end{proof}

\subsection{Proof of Correctness of the Encoding}
\label{app:affinelambda}
We now show our encoding of the affine $ \lambda $-calculus captures
$ \beta \eta $-equivalence.

\subsubsection{Proof of Soundness}
First, let us notice that to showing an equality
$\transl M^o \similarProcesses \transl N^o$ is equivalent to showing
the equalities $\transl M^o_i \similarProcesses \transl N^o_i$ for all
$i \in \CompType  \tau $ where $ \tau $ is the return type of $M$ and $N$.

\begin{lemma}\label{lem:linlambda-substitution}
  Given $\Gamma, x:\tau_1 \vdash M : \tau_2$ and $\Delta \vdash N : \tau_2$, and $i \in \CompType { \tau _2}$, we have:
  $$\transl {M\subst x {N}}_i^o \similarProcesses  \Interact x y {\transl {M}_i^o} {\transl{N}^{y}}.$$
\end{lemma}
\begin{proof}
  By induction. Let us detail a few cases:
  \begin{itemize}
  \item If $M = x$:
    $$
    \begin{aligned}
      \shareInteract x y {} {\transl {x}^o_i}
      {\transl {N}^y}
      &\similarProcesses
      \shareInteract x y {}
      {(\Output x i.\, \Forwarder x o {})}
      {\InputII y {j \in \CompType{ \tau _2}}
        {\transl {N}^y_j}}\\
      &\similarProcesses
      \shareInteract x y {}
      {\Forwarder x o}
      {\transl {N}^y_i}
      \\
      &\similarProcesses \transl {N}^o_i
    \end{aligned}$$
  \item If $M = w \neq x$:
    $$
    \begin{aligned}
      \shareInteract x y {} {\transl {w}^o_i}
      {\transl {N}^y}
      &\similarProcesses
      \shareInteract x y {}
      {(\Output w i.\, \Forwarder w o {})}
      {\transl {N}^y}\\
      &\similarProcesses
      \Output w i.\, (\Forwarder w o {} \parallel \multicut {x\, y} {\transl {N}^y})\\
      &\similarProcesses \transl {y}^o
    \end{aligned}$$

    The second equality is due to the fact that $x$ does not occur in
    the left-hand side of $ \odot $ and the right-handside of
    $ \odot $ starts with an input of $y$ and the last equality due to
    the rule for deadlock ($\transl {N}^y$ starts by an input on $y$).
    
  \item If $M =  \lambda w.\, M'$:
    $$
    \begin{aligned}
      \shareInteract x y {}
      {(\Naming o {w, o}.\, \transl {M'}^o_i)}
      {\transl N^y}
      &\similarProcesses
      \Naming o {w, o}.\,
        \left(\shareInteract x y {} {\transl {M'}^o_i} {\transl N^y}\right)\\
      &\similarProcesses
       \transl { \lambda w.\, M'\subst x N}^o_i
    \end{aligned}$$
  \end{itemize}
\end{proof}

\begin{lemma}
  Consider $ \Gamma   \vdash  M =_{ \beta  \eta } N :  \tau $. Then
  $\transl t^a \ \similarProcesses \transl u^a$.
\end{lemma}
\begin{proof}
  By induction on the definiton of $=_{ \beta  \eta }$. We detail some interesting case:
  
  \begin{itemize}
  \item The case $( \lambda x.\, M)\, N =_{ \beta  \eta } M\subst x N$. Using
    Lemma~\ref{lem:linlambda-substitution}, we have for all $i \in \CompType { \tau }$:

    $$
    \begin{aligned}
      \transl {( \lambda x.\, M)\, N}^o_i
      &\similarProcesses
      \shareInteract x y {}
      {(\Split o {x, o} {\Naming o {x, o}.\, \transl M^o_i})}
      {\transl N^y} \\
      &\similarProcesses
      \shareInteract x y {}
      {\transl M^o_i} {\transl N^y}
      \similarProcesses \transl {M \subst x N}^o_i
    \end{aligned}$$
\item The case $\lambda x.\, M\, x =_{ \beta  \eta }  t$ when $M$ has type $A  \multimap  B$.

  $$
  \begin{aligned}
    \transl { \lambda x.\, M\, x}^o_i &\similarProcesses
    \Naming o {x, o}.\,
    (\shareInteract u v {}
    {\Split {o} {u, o} {\transl M^o_i}}
    {\transl x^v}) \\
    &\similarProcesses
    \Naming o {x, o}.\,
    (\shareInteract u v {}
    {\Split {o} {u, o} {\transl M^o_i}}
    {\transl x^v}) \\
  \end{aligned}$$
  Now, since naming actions float freely, we can assume that $\transl M^o_i \similarProcesses \Naming o {u, o}.\, P$, and we get:
  
  $$
  \begin{aligned}
    \transl { \lambda x.\, M\, x}^o_i &\similarProcesses
    \Naming o {x, o}.\,
    (\shareInteract u v {}
    P
    \Forwarder{x}{v}{}) \\
    &\similarProcesses
    \transl { \lambda x.\, M\, x}^o_i \similarProcesses
    \Naming o {x, o}.\, P \subst u x \similarProcesses \transl M^o_i
  \end{aligned}$$
\end{itemize}
\end{proof}

\subsubsection{Proof of Completeness} We shall now prove
completeness. First, let us define $ \beta  \eta $-long normal forms. We
introduce two judgements $ \Gamma   \vdash _{nf} t: A$ ($t$ is a normal form of type
$A$) and $ \Gamma   \vdash _{ne} t: A$ ($t$ is a neutral term of type $A$). The
rules are as follows:

\begin{mathpar}
  \infer{ \Gamma   \vdash _{nf}  \lambda x.\, t : A  \multimap  B} { \Gamma , x:A  \vdash _{nf} t: B}
  \and
  \infer{ \Gamma   \vdash _{nf} \ttrue,\ffalse  : \linlamBool} {}
  \and
  \infer{ \Gamma   \vdash _{nf} \ifSyntax n t u  : \linlamBool} { \Gamma   \vdash _{ne} n : \linlamBool\and  \Gamma   \vdash _{nf} t,u : \linlamBool }
  \and
  \infer{ \Gamma , x: A  \vdash _{ne} x : A}{}
  \and
  \infer{ \Gamma   \vdash _{ne} n\, t : B}{ \Gamma   \vdash _{ne} n : A  \multimap  B \and  \Gamma   \vdash _{nf} t: A}
\end{mathpar}
\begin{lemma}
  Let $ \Gamma   \vdash  t, u : A$ be two normal forms. Then $t =_{ \beta  \eta } u$ iff $t$
  and $u$ are $ \alpha $-equivalent.
\end{lemma}
\begin{proof}
  Immediate since normal forms cannot be $ \beta $-reduced or $ \eta $-expanded.
\end{proof}
\begin{lemma}\label{lemma:nf_equal}
  For every term $ \Gamma   \vdash  t: A$, there exists a normal form
  $ \Gamma   \vdash  nf(t) : A$ such that $t =_{ \beta  \eta } nf(t)$.
\end{lemma}
\begin{proof}
  By $ \beta $-normalisation and $ \eta $-expansion.
\end{proof}

\begin{lemma}\label{lemma:nf_iso}
  Consider two normal forms $ \Gamma   \vdash _{nf} M, N : A$. Then $ \llbracket M \rrbracket  \cong   \llbracket N \rrbracket$
  implies that $M$ and $N$ are $ \alpha $-equivalent.
\end{lemma}
\begin{proof}
  Standard result on game semantics, done by induction on $M$ and look
  at the first positive move of $ \llbracket M \rrbracket  \cong   \llbracket N \rrbracket$.
\end{proof}

\completenessLambda*
\begin{proof}
  We have already proved the direct implication. The converse
  implication is a consequence of Lemmata \ref{lemma:nf_iso} and \ref{lemma:nf_equal}.
\end{proof}
%%% Local Variables:
%%% mode: latex
%%% TeX-master: "main"
%%% End:
