# Supplementary material for: Game Semantics: Easy as Pi
Source: arXiv:2011.05248 source file (2020-11-10)
Supplement: Supplementary file 3 [file appendix-nondet.tex]

\section{Proofs of \S~\ref{sec:nondet}}

\subsection{Proofs of \S~\ref{sec:dill}}

\soundnessPreorder*
\begin{proof}
  Note that if $ \sigma  \belowStrategies{}  \sigma '$ then
  $ \tau   \odot   \sigma \belowStrategies{}  \tau   \odot   \sigma '$. This implies that the first, third
  and last rules are sound. The second rule is trivial.

  The third rules is a consequence that we have the reduction:

  $$(\oc A  \parallel  A \xrightarrow{c_A} \oc A \xrightarrow{d_A} A)\belowStrategies{} ({\oc A  \parallel  A} \profto A)$$
  where the right most strategy is simply the second projection.
  
\end{proof}
\subsection{Proofs of \S~\ref{sec:IPA}}

To prove Theorem~\ref{thm:adequacySC}, we show the following:
\begin{theorem}\label{thm:adequacyIPA}
  For every closed "program" $ \vdash  M :  \mathbb{N} $,
  we have $M  \approx   \llbracket M \rrbracket$, by
  which we mean:
  \begin{enumerate}
  \item If $M = \LetIn {\vec r}{\vec k} {n}$, then $ \llbracket M \rrbracket =  \llbracket n \rrbracket$
  \item If $M  \rightarrow  N$ then $ \llbracket M \rrbracket \belowProc  \llbracket N \rrbracket$
  \item If $ \llbracket M \rrbracket =  \llbracket n \rrbracket$ then $M  \rightarrow ^* \LetIn {\vec r}{\vec k} {n}$
  \item If $ \llbracket M \rrbracket \belowStrategies {}  \sigma $ then $M  \rightarrow ^* N$ and
    %    $ \llbracket N \rrbracket \weakIso  \sigma $.
        $ \llbracket N \rrbracket \approx  \sigma $.
  \end{enumerate}
\end{theorem}
Theorem~\ref{thm:adequacySC} follows then by composing the
bisimulations together.

\subsubsection{Soundness}
The first point is straightforward, so we focus on the second one.

Given a context $ \Gamma $ containing only locations , and a memory state
$ \rho : \dom \Gamma  \rightarrow   \mathbb{N} $, we define
$\MemStrat^ \rho _ \Gamma  \eqdef  \parallel _{r \in  \Gamma } \MemStrat^{ \rho (r)}_{\bar r}$.

Given a "program" $ \Gamma   \vdash  M :  \mathbb{N} $ and $ \rho  : \dom  \Gamma   \rightarrow   \mathbb{N} $ we write
$\transl {M,  \rho }^o_i$ for $\multicut { \Gamma \, \vec  \Gamma } {
  \transl M^o_i  \parallel \MemStrat^ \rho _ \Gamma }$.

\begin{lemma}\label{lemma:ipa_context}
  Consider that
  $\transl {M,  \rho }^o_i \belowProc \transl{M',  \rho '}^o_i$. Then $\transl
  {E[M],  \rho }^o_i \belowProc \transl {E[M'],  \rho' }^o_i$.
\end{lemma}
\begin{proof}
  By induction on $E$.
  \begin{itemize}
  \item If $E[M] = M; N$: then we have
$$
\begin{aligned}
  \transl {M; N,  \rho }^o_i &\similarProcesses
  \multicut { \Gamma \, \bar  \Gamma } {
    \shareInteract x y { \Gamma }
      {\transl M^x_{\Start}}
      {\Wait y {\transl N^o_i}}
      \parallel \MemStrat^ \rho _ \Gamma 
    } \\
    &\similarProcesses
    \multicut {x\, y;  \Gamma \, \bar  \Gamma } {
      {\transl M^x_\Start \parallel \MemStrat^ \rho _ \Gamma  \parallel_ \Gamma  \Wait y {\transl N^o_i}}
    } \\
    &\belowProc
    \multicut {x\, y;  \Gamma \, \bar  \Gamma } {
      {\transl {M'}^x_\Start \parallel \MemStrat^ {\rho'} _ \Gamma  \parallel_ \Gamma  \Wait y {\transl N^o_i}}
    } \\
    &\similarProcesses
    \transl {M'; N, \rho'}^o_i
  \end{aligned}$$
\item Other cases are similar.
  \end{itemize}

\end{proof}

\begin{lemma}
  Consider "programs" $ \Gamma  \vdash M, N : \mathbb{N} $. Then, for any
  $ \rho  : \dom  \Gamma   \rightarrow   \mathbb{N} $ if $ \langle M,  \rho  \rangle  \rightarrow ^*  \langle N,  \rho  \rangle $, then
  $\transl {M,  \rho }^o_i \belowProc \transl {N,  \rho }^o_i$.
\end{lemma}
\begin{proof}
  First, without loss of generality by soundness of the PCF
  translation, we can assume that $M$ and $N$ are in normal form for
  $ \rightarrow _{\PCF}$.

  We detail a few rules:
  \begin{itemize}
  \item The rule for reading from a location: $M = \oc r$, $N =  \rho (r) = k$.
    Then we have:
    $$
    \begin{aligned}
      \multicut {r\, \bar r}{\transl {\oc r}^o_i  \parallel  \MemStrat_ {\bar r}^ k}
      &\similarProcesses
      \multicut {r\, \bar r}{
        (\Der r x.\, \Output x \ReadMsg.\, \Forwarder x o {})
        \parallel \MemStrat^k_{\bar r}} \\
      &\belowProc
      \multicut {x\, y; r\, \bar r}{
      (\Output x {\ReadMsg}.\, \Forwarder r o {})
      \parallel \InputII y {} {\ReadMsg: \Output y k.\, \MemStrat^k_{\bar r}; ...}} \\
    &\similarProcesses \multicut {r\, \bar r}{\Output o k \parallel \MemStrat^k_{\bar r}}
    \end{aligned}$$
  The rule for assignment has a similar proof.
\item The rule
  $ \langle E[M], \rho \rangle \rightarrow \langle E[M'], \rho '
  \rangle $ with
  $ \langle M, \rho \rangle \rightarrow \langle M', \rho ' \rangle $
  is a consequence of Lemma \ref{lemma:ipa_context}.
  \end{itemize}
\end{proof}

\subsubsection{Adequacy} To prove adequacy,we first need to define
some kind of Bohm trees of terms of $\PCFWM$ by reducing all possible
redexes $ \rightarrow _{\PCF}$. Given a term $M$ we define its Bohm tree $\BT M$
as follows:

$$\BT M \eqdef \left\{
\begin{aligned}
  &\bot \qquad && \text{if $M$ does not have a head normal form for $ \rightarrow _{\PCF}$} \\
  &\oc r \qquad && \text{If $M  \rightarrow ^*_{\PCF} \oc r$} \\
  & r := \BT N \qquad && \text{If $M  \rightarrow ^*_{\PCF} r := N$}\\
  & \mathsf{succ}(N) \qquad && \text{If $M  \rightarrow ^*_{\PCF} \mathsf{succ}(N)$}\\
  & \mathsf{iszero}(N) \qquad && \text{If $M  \rightarrow ^*_{\PCF} \mathsf{iszero}(N)$}\\
  & r := \BT N \qquad && \text{If $M  \rightarrow ^*_{\PCF} r := N$}\\
  & \BT {N_1}; \BT {N_2} \qquad && \text{If $M  \rightarrow ^*_{\PCF} N_1; N_2$}\\
  & \BT {N_1}  \parallel  \BT {N_2} \qquad && \text{If $M  \rightarrow ^*_{\PCF} N_1  \parallel  N_2$}\\
  & \LetIn r k {\BT N} \qquad && \text{If $M  \rightarrow ^*_{\PCF} \LetIn r k {\BT N}$}\\
  & \ifte {\BT M} {\BT {N_1}} {\BT {N_2}} \qquad && \text{If $M  \rightarrow ^*_{\PCF} \ifte {\BT M} {\BT {N_1}} {\BT {N_2}}$}\\
\end{aligned}\right.$$
Note that the head normal form cannot be a variable, a
$ \lambda $-abstraction or an application because $M$ is a
program. Bohm trees are in general infinite.
\begin{lemma}
  For any program $M$, we have $\transl M^o \similarProcesses \transl {\BT M}^o$.
\end{lemma}

A \textbf{normal form} a program $M$ such that $\BT M = M$.  The
adequacy result follows from this result. Let us write $ \llbracket  \langle M,  \rho  \rangle  \rrbracket$ for
$ \llbracket \transl { \langle M,  \rho  \rangle }^o_\Start \rrbracket$.

To prove the adequacy result, we will rely on this result:
\begin{lemma}\label{lemma:technical}
  Consider a minimal event of
  $ \llbracket \shareInteract a b  \Delta  P {\InputII b {i \in I} {Q_i}} \rrbracket$ where the type
  of $A$ is $\oplus_{i \in I} T_i$. It is either:
  \begin{itemize}
  \item A minimal event of $ \llbracket P \rrbracket$ not on $a$
  \item A minimal event of $ \llbracket Q_k \rrbracket$, and $ \llbracket P \rrbracket$ has an initial event
    output $k$ to $a$.
  \end{itemize}
\end{lemma}
\begin{proof}
  This is a simple reasoning on the composition. $ \llbracket P \rrbracket$ and $ \llbracket Q \rrbracket$
  synchronise on $ \llbracket \oplus_{i \in I} T_i$ which means that a most $ \llbracket P \rrbracket$
  sends a move to $ \llbracket Q \rrbracket$. As a result, a minimal move of the process is either:
  \begin{itemize}
  \item A minimal move of $ \llbracket P \rrbracket$ before any move on $a$
  \item A move of $ \llbracket P \rrbracket$ straight after a move on $a$ -- impossible by
    courtesy. ($a$ is positive)
  \item A move of $ \llbracket \InputII b {i \in I} {i.\, Q_i} \rrbracket$ after a
    reception on $b$, ie. a minimal move of $ \llbracket Q_k \rrbracket$. Moreover, if that
    the case, then the causal history of this move in the interaction
    contains an output from $P$ on $a$ as desired. By courtesy this
    move must be minimal.
  \end{itemize}

\end{proof}
\begin{lemma}
  Let $ \Gamma \vdash M : A$ be a "program" of base type $A$ and
  $ \rho : \dom \Gamma \rightarrow \mathbb{N} $ a memory
  state. Consider $e$ a minimal event of
  $ \llbracket\langle M, \rho \rangle \rrbracket$.
  \begin{itemize}
  \item If $e$ is a neutral event, then there exists a reduction
    $ \langle M,  \rho  \rangle   \rightarrow ^*  \langle M' \c{}   \rho ' \rangle $ with $ \llbracket \langle M',  \rho ' \rangle \rrbracket \approx  \llbracket  \langle M,  \rho  \rangle  \rrbracket/e $
  \item If $e$ is a value $v$ of $A$, then $ \langle M,  \rho  \rangle   \rightarrow ^*  \langle \LetIn {\vec r}{\vec k} v,  \rho ' \rangle $.
  \end{itemize}
\end{lemma}
\begin{proof}
  Without loss of generality, we can assume that $M$ is a normal
  form. Moreover, since we know
  that $e$ is a minimal event of $ \llbracket  \langle M,  \rho  \rangle  \rrbracket$ by continuity, there must
  exist a finite approximation $M_n$ (ie. $M$ where branches deeper
  than $n$ are cut) of $M$ such that $ \llbracket  \langle M_n,  \rho  \rangle  \rrbracket$ contains $e$. We
  then proceed by induction on $M_n$.

  We detail a few cases, but most are similar using Lemma \ref{lemma:technical}:

  \begin{itemize}
  \item If $M = \oc N$, then there are two cases:
    \begin{itemize}
    \item Either $e = n$: then by induction we know that $ \langle N,  \rho  \rangle $ must
      normalise to $ \langle r,  \rho ' \rangle $. Then $ \langle M,  \rho  \rangle   \rightarrow ^*  \langle  \rho '(r),  \rho ' \rangle $.
    \item Or $e$ is an internal event. Then $e$ corresponds to an
      internal event of $ \llbracket\langle N, \rho \rangle \rrbracket$ so by
      induction, $ \langle N,  \rho  \rangle $ reduces to $ \langle N',  \rho ' \rangle $, and the desired state
      is $ \langle \oc N',  \rho ' \rangle $.
    \end{itemize}
  \item $M = \LetIn r k N$. Then we directly apply the induction
    hypothesis to $ \langle N,  \rho [r := k] \rangle $.
  \item $N  \parallel  N'$. We us Lemma \ref{lemma:technical}. There are two main cases:
    \begin{itemize}
    \item If the minimal event is in $ \llbracket N \rrbracket  \parallel   \llbracket N' \rrbracket$, then we apply the induction hypothesis
    \item Otherwise, it must be that $ \llbracket N \rrbracket$ and $ \llbracket N' \rrbracket$ both have an
      initial event outputting $\Done$, and by induction we know that
      $N$ and $N'$ reduce to $\SkipTerm$ and then we can conclude.
    \end{itemize}
    \end{itemize}
\end{proof}

From this result, Theorem \ref{thm:adequacyIPA} follows.

%%% Local Variables:
%%% mode: latex
%%% TeX-master: "main"
%%% End:
